# Supplementary material for: Network-Aware Scheduling for Remote Gate Execution in Quantum Data Centers
Source: arXiv:2504.20176 source file (2025-04-28)
Supplement: Supplementary file 1 [file Appendix.tex]

\section{Appendix}

Figure \ref{fig:appendix_gates_per_layer} shows the number of two-qubit gates per layer in the DAG representation of various transpiled circuits. The QFT circuit has significantly fewer two-qubit gates per layer compared to the other circuits. Notably, increasing the number of qubits in QFT primarily increases the number of layers in the DAG, but each layer still contains only a small number of two-qubit gates. This behavior helps explain the similar execution delays observed for QFT under both dynamic and static schedulers, as limited parallelism reduces the advantage of dynamic scheduling.

\begin{figure}
\centering
    \includegraphics[width=5cm]%{img/delay_as_bw.pdf}
    {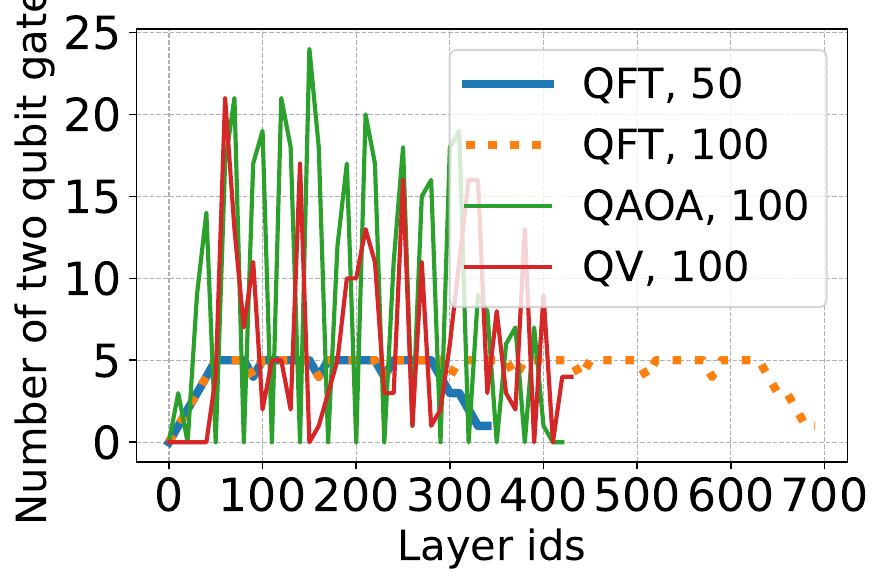}
    \vspace{-0.06in}
%\captionsetup{justification=centering} 
  \caption{Number of two qubit gates in each layer of different circuits. Circuits with higher number of gates per layer can benefit from dynamic scheduler.}\label{fig:appendix_gates_per_layer}
\end{figure}
